# Supplementary material for: Cumulant Green's function methods for molecules
Source: arXiv:2402.16414 ancillary file (2024-02-26)
Supplement: Supplementary file 1 [file si.pdf]

# Cumulant Green's function methods for molecules

Pierre-François Loos,[a)] Antoine Marie,[b)] and Abdallah Ammar[c)]
*Laboratoire de Chimie et Physique Quantiques (UMR 5626), Université de Toulouse, CNRS, UPS, France*

This document contains a detailed derivation of the cumulant expansion. Notations are defined in the main manuscript.

## I. RETARDED ONE-BODY GREEN'S FUNCTION

The matrix elements of the Hartree-Fock (HF) retarded Green's function in the time domain are

$$G_{pq}^{\text{HF}}(t) = -\mathrm{i}\,\Theta(t)\,e^{-\mathrm{i}\epsilon_p^{\text{HF}} t}\,\delta_{pq} \tag{1}$$

Thanks to the following definition of the Heaviside step function

$$\Theta(t) = -\frac{1}{2\pi\mathrm{i}} \int_{-\infty}^{\infty} \mathrm{d}\omega \frac{e^{-\mathrm{i}\omega t}}{\omega + \mathrm{i}\eta} \tag{2}$$

one can compute the Fourier transform of Eq. (1) and obtain the expression of the matrix elements in the frequency domain

$$\begin{aligned}
G_{pq}^{\text{HF}}(\omega) &= \int \mathrm{d}t\, e^{\mathrm{i}\omega t}\, G_{pr}^{\text{HF}}(t) \\
&= -\mathrm{i}\,\delta_{pq} \int_{-\infty}^{\infty} \mathrm{d}t\, e^{\mathrm{i}\left(\omega - \epsilon_p^{\text{HF}}\right)t}\, \Theta(t) \\
&= -\mathrm{i}\,\delta_{pq} \int_{-\infty}^{\infty} \mathrm{d}t\, e^{\mathrm{i}\left(\omega - \epsilon_p^{\text{HF}}\right)t} \left[ -\frac{1}{2\pi\mathrm{i}} \int_{-\infty}^{\infty} \mathrm{d}\omega' \frac{e^{-\mathrm{i}\omega' t}}{\omega' + \mathrm{i}\eta} \right] \\
&= \frac{1}{2\pi}\,\delta_{pq} \int_{-\infty}^{\infty} \mathrm{d}\omega' \frac{1}{\omega' + \mathrm{i}\eta} \int_{-\infty}^{\infty} \mathrm{d}t\, e^{\mathrm{i}\left(\omega - \omega' - \epsilon_p^{\text{HF}}\right)t} \\
&= \frac{1}{2\pi}\,\delta_{pq} \int_{-\infty}^{\infty} \mathrm{d}\omega' \frac{1}{\omega' + \mathrm{i}\eta}\,(2\pi)\,\delta\!\left(\omega - \omega' - \epsilon_p^{\text{HF}}\right) \\
&= \frac{\delta_{pq}}{\omega - \left(\epsilon_p^{\text{HF}} - \mathrm{i}\eta\right)}.
\end{aligned} \tag{3}$$

## II. CUMULANT

The general definition of the cumulant, obtained by equating the first-order term in $W$ (refer to the manuscript), is expressed as

$$G^{\text{HF}}(t) C(t) = \iint \mathrm{d}t_1\, \mathrm{d}t_2\, G^{\text{HF}}(t - t_1) \Sigma^{\text{c}}(t_1 - t_2) G^{\text{HF}}(t_2) \tag{4}$$

Projecting this equation in the spinorbital basis yields

$$\begin{aligned}
\sum_r G_{pr}^{\text{HF}}(t) C_{rq}(t) &= \sum_{rs} \iint \mathrm{d}t_1\, \mathrm{d}t_2\, G_{pr}^{\text{HF}}(t - t_1) \Sigma_{rs}^{\text{c}}(t_1 - t_2) G_{sq}^{\text{HF}}(t_2) \\
\Rightarrow -\mathrm{i} \sum_r \Theta(t)\, e^{-\mathrm{i}\epsilon_p^{\text{HF}} t} \delta_{pr}\, C_{rq}(t) &= \sum_{rs} \iint \mathrm{d}t_1\, \mathrm{d}t_2\, G_{pr}^{\text{HF}}(t - t_1) \Sigma_{rs}^{\text{c}}(t_1 - t_2) G_{sq}^{\text{HF}}(t_2) \\
\Rightarrow -\mathrm{i}\,\Theta(t)\, e^{-\mathrm{i}\epsilon_p^{\text{HF}} t}\, C_{pq}(t) &= \sum_{rs} \iint \mathrm{d}t_1\, \mathrm{d}t_2\, G_{pr}^{\text{HF}}(t - t_1) \Sigma_{rs}^{\text{c}}(t_1 - t_2) G_{sq}^{\text{HF}}(t_2) \\
\Rightarrow \Theta(t)\, C_{pq}(t) &= \mathrm{i}\, e^{\mathrm{i}\epsilon_p^{\text{HF}} t} \sum_{rs} \iint \mathrm{d}t_1\, \mathrm{d}t_2\, G_{pr}^{\text{HF}}(t - t_1) \Sigma_{rs}^{\text{c}}(t_1 - t_2) G_{sq}^{\text{HF}}(t_2)
\end{aligned} \tag{5}$$

---

[a)]Electronic mail: loos@irsamc.ups-tlse.fr
[b)]Electronic mail: amarie@irsamc.ups-tlse.fr
[c)]Electronic mail: aammar@irsamc.ups-tlse.fr

Assuming $t$ to be positive, we obtain

$$C_{pq}(t) = \mathrm{i} \int \frac{\mathrm{d}\omega}{2\pi} \, e^{-\mathrm{i}(\omega-\epsilon_p^{\text{HF}})t} \, G_{pp}^{\text{HF}}(\omega) \, \Sigma_{pq}^{\text{c}}(\omega) \, G_{qq}^{\text{HF}}(\omega) \tag{6}$$

Using the diagonal approximation $\Sigma_{pq}(\omega) \approx \delta_{pq}\Sigma_{pp}(\omega)$ leads to

$$\begin{aligned} C_{pq}(t) &= \mathrm{i}\,\delta_{pq} \int \frac{\mathrm{d}\omega}{2\pi} \, e^{-\mathrm{i}(\omega-\epsilon_p^{\text{HF}})t} \left[G_{pp}^{\text{HF}}(\omega)\right]^2 \Sigma_{pp}^{\text{c}}(\omega) \\ &= \mathrm{i}\,\delta_{pq} \int \frac{\mathrm{d}\omega}{2\pi} \, e^{-\mathrm{i}(\omega-\epsilon_p^{\text{HF}})t} \, \Sigma_{pp}^{\text{c}}(\omega) \left[\frac{1}{\omega - \left(\epsilon_p^{\text{HF}} - \mathrm{i}\eta\right)}\right]^2 \\ &= \mathrm{i}\,\delta_{pq} \int \frac{\mathrm{d}\omega}{2\pi} \, e^{-\mathrm{i}\omega t} \, \frac{\Sigma_{pp}^{\text{c}}\left(\omega + \epsilon_p^{\text{HF}}\right)}{\left[\omega - (0 - \mathrm{i}\eta)\right]^2} \end{aligned} \tag{7}$$

Inserting the frequency expression of the self-energy

$$\Sigma_{pp}^{\text{c}}\left(\omega + \epsilon_p^{\text{HF}}\right) = \sum_{i\nu} \frac{M_{pi\nu}^2}{\omega - \Delta_{pi\nu}} + \sum_{a\nu} \frac{M_{pa\nu}^2}{\omega - \Delta_{pa\nu}} \tag{8}$$

with

$$\Delta_{pi\nu} = \epsilon_i - \epsilon_p^{\text{HF}} - \Omega_\nu - \mathrm{i}\eta \qquad\qquad \Delta_{pa\nu} = \epsilon_a - \epsilon_p^{\text{HF}} + \Omega_\nu - \mathrm{i}\eta \tag{9}$$

we obtain

$$\begin{aligned} C_{pp}(t) &= \mathrm{i} \sum_{i\nu} M_{pi\nu}^2 \int \frac{\mathrm{d}\omega}{2\pi} \, e^{-\mathrm{i}\omega t} \, \frac{1}{\left[\omega - (0 - \mathrm{i}\eta)\right]^2} \, \frac{1}{\omega - \Delta_{pi\nu}} \\ &+ \mathrm{i} \sum_{a\nu} M_{pa\nu}^2 \int \frac{\mathrm{d}\omega}{2\pi} \, e^{-\mathrm{i}\omega t} \, \frac{1}{\left[\omega - (0 - \mathrm{i}\eta)\right]^2} \, \frac{1}{\omega - \Delta_{pa\nu}}. \end{aligned} \tag{10}$$

Applying the residue theorem on the following integral [where $\text{Im}(\omega_1), \text{Im}(\omega_2) < 0$] leads to

$$\begin{aligned} \int \frac{\mathrm{d}\omega}{2\pi} \, e^{-\mathrm{i}\omega t} \, \frac{1}{(\omega - \omega_1)^2} \, \frac{1}{\omega - \omega_2} &= (-\mathrm{i}) \left\{ \left[\partial_\omega\left(\frac{e^{-\mathrm{i}\omega t}}{\omega - \omega_2}\right)\right]_{\omega=\omega_1} + \left[\frac{e^{-\mathrm{i}\omega t}}{(\omega - \omega_1)^2}\right]_{\omega=\omega_2} \right\} \\ &= \frac{(-\mathrm{i})}{(\omega_1 - \omega_2)^2} \left\{ \left[(-\mathrm{i}t)(\omega_1 - \omega_2) - 1\right] e^{-\mathrm{i}\omega_1 t} + e^{-\mathrm{i}\omega_2 t} \right\}, \end{aligned} \tag{11}$$

we find

$$\int \frac{\mathrm{d}\omega}{2\pi} \, e^{-\mathrm{i}\omega t} \, \frac{1}{\left[\omega - (0 - \mathrm{i}\eta)\right]^2} \, \frac{1}{\omega - \Delta_{pi\nu}} = \frac{-\mathrm{i}}{\Delta_{pi\nu}^2}\left(e^{-\mathrm{i}\Delta_{pi\nu} t} + \mathrm{i}\Delta_{pi\nu} t - 1\right) \tag{12}$$

and

$$\int \frac{\mathrm{d}\omega}{2\pi} \, e^{-\mathrm{i}\omega t} \, \frac{1}{\left[\omega - (0 - \mathrm{i}\eta)\right]^2} \, \frac{1}{\omega - \Delta_{pa\nu}} = \frac{-\mathrm{i}}{\Delta_{pa\nu}^2}\left(e^{-\mathrm{i}\Delta_{pa\nu} t} + \mathrm{i}\Delta_{pa\nu} t - 1\right). \tag{13}$$

Therefore, the diagonal elements of the cumulant are given by the following expression

$$\begin{aligned} C_{pp}(t) &= \sum_{i\nu} \frac{M_{pi\nu}^2}{\Delta_{pi\nu}^2} \left(e^{-\mathrm{i}\Delta_{pi\nu} t} + \mathrm{i}\Delta_{pi\nu} t - 1\right) + \sum_{a\nu} \frac{M_{pa\nu}^2}{\Delta_{pa\nu}^2} \left(e^{-\mathrm{i}\Delta_{pa\nu} t} + \mathrm{i}\Delta_{pa\nu} t - 1\right) \\ &= \sum_{i\nu} \zeta_{pi\nu} \left(e^{-\mathrm{i}\Delta_{pi\nu} t} + \mathrm{i}\Delta_{pi\nu} t - 1\right) + \sum_{a\nu} \zeta_{pa\nu} \left(e^{-\mathrm{i}\Delta_{pa\nu} t} + \mathrm{i}\Delta_{pa\nu} t - 1\right), \end{aligned} \tag{14}$$

where we have introduced the following intermediate quantities:

$$\zeta_{pi\nu} = \left(\frac{M_{pi\nu}}{\Delta_{pi\nu}}\right)^2, \qquad\qquad \zeta_{pa\nu} = \left(\frac{M_{pa\nu}}{\Delta_{pa\nu}}\right)^2. \tag{15}$$

## III. LANDAU FORM

In this section, we derive the Landau form of the cumulant. The first step is to derive the spectral representation of the self-energy

$$\begin{aligned}\Sigma^{\text{c}}_{pp}(\omega) &= \text{Re}[\Sigma^{\text{c}}_{pp}(\omega)] + \text{i}\,\text{Im}[\Sigma^{\text{c}}_{pp}(\omega)] \\ &= \frac{1}{\pi}\mathcal{P}\int \text{d}\omega' \frac{\text{Im}[\Sigma^{\text{c}}_{pp}(\omega')]}{\omega' - \omega} + \text{i}\int \text{d}\omega'\, \text{Im}[\Sigma^{\text{c}}_{pp}(\omega')]\delta(\omega' - \omega) \\ &= \frac{1}{\pi}\int \text{d}\omega' \frac{\text{Im}[\Sigma^{\text{c}}_{pp}(\omega')]}{\omega' - \omega - \text{i}\eta} = \int \text{d}\omega' \,\frac{\beta_p(\omega')}{\omega - \omega' + \text{i}\eta}.\end{aligned} \tag{16}$$

To obtain this expression, we first used the Kramers-Kronig relation, then the identity

$$\frac{1}{x \pm \text{i}\eta} = \mathcal{P}\left(\frac{1}{x}\right) \mp \text{i}\,\pi\,\delta(x), \tag{17}$$

and finally we introduced

$$\beta_p(\omega) = -\frac{1}{\pi}\,\text{Im}\,\Sigma^{\text{c}}_{pp}(\omega) \tag{18}$$

This expression of the self-energy is now inserted into the cumulant

$$\begin{aligned}C_{pq}(t) &= \text{i}\,\delta_{pq}\int \frac{\text{d}\omega}{2\pi}\, e^{-\text{i}\omega t}\, \frac{\Sigma^{\text{c}}_{pp}\left(\omega + \epsilon^{\text{HF}}_p\right)}{[\omega - (0 - \text{i}\eta)]^2} \\ &= \text{i}\,\delta_{pq}\int \frac{\text{d}\omega}{2\pi}\,\frac{e^{-\text{i}\omega t}}{[\omega - (0 - \text{i}\eta)]^2}\int \text{d}\omega'\,\frac{\beta_p(\omega')}{\omega + \epsilon^{\text{HF}}_p - \omega' + \text{i}\eta} \\ &= \frac{\text{i}\,\delta_{pq}}{2\pi}\int \text{d}\omega'\,\beta_p(\omega')\int \text{d}\omega\,\frac{e^{-\text{i}\omega t}}{[\omega - (0 - \text{i}\eta)]^2\left[\omega - \left(\omega' - \epsilon^{\text{HF}}_p - \text{i}\eta\right)\right]} \\ &= \frac{\text{i}\,\delta_{pq}\,(-2\pi\text{i})}{2\pi}\int \text{d}\omega'\,\beta_p(\omega')\left[\partial_\omega\left\{\frac{e^{-\text{i}\omega t}}{\left[\omega - \left(\omega' - \epsilon^{\text{HF}}_p - \text{i}\eta\right)\right]}\right\}_{\omega = -\text{i}\eta} + \left(\frac{e^{-\text{i}\omega t}}{(\omega + \text{i}\eta)^2}\right)_{\omega = \omega' - \epsilon^{\text{HF}}_p - \text{i}\eta}\right] \\ &= \delta_{pq}\int \text{d}\omega'\,\beta_p(\omega')\left[\frac{\text{i}t\left(\omega' - \epsilon^{\text{HF}}_p\right) - 1}{\left(\omega' - \epsilon^{\text{HF}}_p\right)^2} + \frac{e^{-\text{i}\left(\omega' - \epsilon^{\text{HF}}_p - \text{i}\eta\right)t}}{\left(\omega' - \epsilon^{\text{HF}}_p\right)^2}\right] \\ &= \delta_{pq}\int \text{d}\omega\,\frac{\beta_p\left(\omega + \epsilon^{\text{HF}}_p\right)}{\omega^2}\left(e^{-\text{i}\omega t} + \text{i}\omega t - 1\right).\end{aligned} \tag{19}$$

which yields the so-called Landau form of the cumulant.

## IV. $GW$+C PROPAGATOR

The $GW$+C ansatz in the time domain reads

$$\begin{aligned}G_{pp}(t) &= G^{\text{HF}}_{pp}(t)\,\exp\left[C_{pp}(t)\right] \\ &= -\text{i}\,\Theta(t)\,\exp\left[-\text{i}\epsilon^{\text{HF}}_p t + C_{pp}(t)\right] \\ &= -\text{i}\,\Theta(t)\,\exp\left[-\text{i}\epsilon^{\text{HF}}_p t + \sum_{iv}\zeta_{piv}\left(e^{-\text{i}\Delta_{piv}t} + \text{i}\Delta_{piv}t - 1\right) + \sum_{av}\zeta_{pav}\left(e^{-\text{i}\Delta_{pav}t} + \text{i}\Delta_{pav}t - 1\right)\right] \\ &= -\text{i}\,\Theta(t)\,Z^{\text{QP}}_p\,\exp\left(-\text{i}\epsilon^{\text{QP}}_p t\right)\,\exp\left(\sum_{iv}\zeta_{piv}\,e^{-\text{i}\Delta_{piv}t} + \sum_{av}\zeta_{pav}\,e^{-\text{i}\Delta_{pav}t}\right)\end{aligned} \tag{20}$$

where the weight of the quasiparticle peak is

$$Z^{\text{QP}}_p = \exp\left(-\sum_{iv}\zeta_{piv} - \sum_{av}\zeta_{pav}\right) \tag{21}$$

and the quasiparticle energy is given by

$$\epsilon_p^{\text{QP}} = \epsilon_p^{\text{HF}} - \left( \sum_{iv} \zeta_{piv}\, \Delta_{piv} + \sum_{av} \zeta_{pav}\, \Delta_{pav} \right) \tag{22}$$

Expanding up to first order and applying the Fourier transform leads to

$$\begin{aligned}
G_{pp}(\omega) &= \int_{-\infty}^{+\infty} \mathrm{d}t\, e^{\mathrm{i}\omega t}\, G_{pp}(t) \\
&= -\mathrm{i}\, Z_p^{\text{QP}} \int_0^{+\infty} \mathrm{d}t\, e^{\mathrm{i}\left(\omega - \epsilon_p^{\text{QP}}\right)t} \exp\left( \sum_{iv} \zeta_{piv}\, e^{-\mathrm{i}\Delta_{piv} t} + \sum_{av} \zeta_{pav}\, e^{-\mathrm{i}\Delta_{pav} t} \right) \\
&\approx -\mathrm{i}\, Z_p^{\text{QP}} \int_0^{+\infty} \mathrm{d}t\, e^{\mathrm{i}\left(\omega - \epsilon_p^{\text{QP}}\right)t} \left( 1 + \sum_{iv} \zeta_{piv}\, e^{-\mathrm{i}\Delta_{piv} t} + \sum_{av} \zeta_{pav}\, e^{-\mathrm{i}\Delta_{pav} t} \right) \\
&= -\mathrm{i}\, Z_p^{\text{QP}} \int_0^{+\infty} \mathrm{d}t\, e^{\left[-\eta + \mathrm{i}\left(\omega - \epsilon_p^{\text{QP}}\right)\right]t} \\
&\quad - \mathrm{i}\, Z_p^{\text{QP}} \sum_{iv} \zeta_{piv} \int_0^{+\infty} \mathrm{d}t\, e^{\left\{-\eta + \mathrm{i}\left[\omega - \left(\epsilon_p^{\text{QP}} + \Delta_{piv}\right)\right]\right\}t} - \mathrm{i}\, Z_p^{\text{QP}} \sum_{av} \zeta_{pav} \int_0^{+\infty} \mathrm{d}t\, e^{\left\{-\eta + \mathrm{i}\left[\omega - \left(\epsilon_p^{\text{QP}} + \Delta_{pav}\right)\right]\right\}t} \\
&= \frac{Z_p^{\text{QP}}}{\omega - \epsilon_p^{\text{QP}} + \mathrm{i}\eta} + \sum_{iv} \frac{Z_{piv}^{\text{sat}}}{\omega - \epsilon_{piv}^{\text{sat}} + \mathrm{i}\eta} + \sum_{av} \frac{Z_{pav}^{\text{sat}}}{\omega - \epsilon_{pav}^{\text{sat}} + \mathrm{i}\eta}
\end{aligned} \tag{23}$$

where we have introduced two sets of satellites at energies

$$\epsilon_{piv}^{\text{sat}} = \epsilon_p^{\text{QP}} + \Delta_{piv}, \qquad \epsilon_{pav}^{\text{sat}} = \epsilon_p^{\text{QP}} + \Delta_{pav}, \tag{24}$$

with the respective weights

$$Z_{piv}^{\text{sat}} = Z_p^{\text{QP}}\, \zeta_{piv}, \qquad Z_{pav}^{\text{sat}} = Z_p^{\text{QP}}\, \zeta_{pav}. \tag{25}$$

## V. SPECTRAL FUNCTION

The diagonal elements of the spectral function are obtained as

$$\begin{aligned}
A_{pp}^{GW+\text{C}}(\omega) &= -\frac{1}{\pi} \operatorname{Im} G_{pp}(\omega) \\
&= -\frac{1}{\pi} \operatorname{Im} \left[ \frac{Z_p^{\text{QP}}}{\omega - \epsilon_p^{\text{QP}} + \mathrm{i}\eta} + \sum_{qv} \frac{Z_{pqv}^{\text{sat}}}{\omega - \epsilon_{pqv}^{\text{sat}} + \mathrm{i}\eta} \right] \\
&= -\frac{1}{\pi} \operatorname{Im} \left[ \frac{\operatorname{Re} Z_p^{\text{QP}} + \mathrm{i} \operatorname{Im} Z_p^{\text{QP}}}{\omega - \operatorname{Re} \epsilon_p^{\text{QP}} + \mathrm{i}\left(\eta - \operatorname{Im} \epsilon_p^{\text{QP}}\right)} + \sum_{qv} \frac{\operatorname{Re} Z_{pqv}^{\text{sat}} + \mathrm{i} \operatorname{Im} Z_{pqv}^{\text{sat}}}{\omega - \operatorname{Re} \epsilon_{pqv}^{\text{sat}} + \mathrm{i}\left(\eta - \operatorname{Im} \epsilon_{pqv}^{\text{sat}}\right)} \right] \\
&= -\frac{1}{\pi} \operatorname{Im} \left[ \frac{\left(\operatorname{Re} Z_p^{\text{QP}} + \mathrm{i} \operatorname{Im} Z_p^{\text{QP}}\right)\left(\omega - \operatorname{Re} \epsilon_p^{\text{QP}} - \mathrm{i}\left(\eta - \operatorname{Im} \epsilon_p^{\text{QP}}\right)\right)}{\left(\omega - \operatorname{Re} \epsilon_p^{\text{QP}}\right)^2 + \left(\operatorname{Im} \epsilon_p^{\text{QP}}\right)^2} + \sum_{qv} \frac{\left(\operatorname{Re} Z_{pqv}^{\text{sat}} + \mathrm{i} \operatorname{Im} Z_{pqv}^{\text{sat}}\right)\left(\omega - \operatorname{Re} \epsilon_{pqv}^{\text{sat}} - \mathrm{i}\left(\eta - \operatorname{Im} \epsilon_{pqv}^{\text{sat}}\right)\right)}{\left(\omega - \operatorname{Re} \epsilon_{pqv}^{\text{sat}}\right)^2 + \left(\operatorname{Im} \epsilon_{pqv}^{\text{sat}}\right)^2} \right] \\
&= -\frac{1}{\pi} \left[ \frac{\left(\operatorname{Re} Z_p^{\text{QP}}\right)\left(\operatorname{Im} \epsilon_p^{\text{QP}}\right) + \left(\operatorname{Im} Z_p^{\text{QP}}\right)\left(\omega - \operatorname{Re} \epsilon_p^{\text{QP}}\right)}{\left(\omega - \operatorname{Re} \epsilon_p^{\text{QP}}\right)^2 + \left(\operatorname{Im} \epsilon_p^{\text{QP}}\right)^2} + \sum_{qv} \frac{\left(\operatorname{Re} Z_{pqv}^{\text{sat}}\right)\left(\operatorname{Im} \epsilon_{pqv}^{\text{sat}}\right) + \left(\operatorname{Im} Z_{pqv}^{\text{sat}}\right)\left(\omega - \operatorname{Re} \epsilon_{pqv}^{\text{sat}}\right)}{\left(\omega - \operatorname{Re} \epsilon_{pqv}^{\text{sat}}\right)^2 + \left(\operatorname{Im} \epsilon_{pqv}^{\text{sat}}\right)^2} \right].
\end{aligned} \tag{26}$$
